# Supplementary material for: Controlled LLM Decoding via Discrete Auto-regressive Biasing
Source: arXiv:2502.03685 source file (2025-02-06)
Supplement: Supplementary file 1 [file diversity_table_sentiment.tex]

\begin{table}[h]
\caption{Sampling Algorithm performance on Sentiment Control task for DBS + DAB, BOLT. While the sentiment control does decline from just using DAB on its own, DBS + DAB still exhibits superior sentiment control as well as improved diversity and efficiency.}
\label{appndx:tab:sentiment-control-div}
\centering

\begin{tabular}{lccccccl}\toprule
      & \textbf{Ext. Clsf} & \textbf{PPL} &\textbf{ Dist-3} & \textbf{Speed} &\textbf{Self-BLEU}\\\midrule
DAB & \textbf{.829} & 15.194 & \textbf{.928} & \textbf{6.1957} & \textbf{.199} \\
BOLT & .795 & \textbf{11.900} & .885 & 11.63 & .305
\\\bottomrule
\end{tabular}
\end{table}
